# Supplementary material for: ARRQP: Anomaly Resilient Real-time QoS Prediction Framework with Graph Convolution
Source: arXiv:2310.02269 source file (2023-09-22)
Supplement: Supplementary file 1 [file 7appendix.tex]

\section{Appendix-A}\label{sec:appendixA}
Here, we discuss the comprehensive details of the multi-head graph attention framework utilized for the comparative model study in Section \ref{subsec:model_study}. Additionally, we give the details of various parameters used in different modules of our framework.

\subsection{Multi-head Graph Attention Framework (MhGAT)}
To give the justification of the importance of the multi-head graph convolution framework without attention, we extend our work by employing an attention mechanism to it.  
% The overall architecture is shown in Figure \ref{fig:mhgat}.

% \begin{figure}
%     \centering
%     \includegraphics[width=\linewidth]{fig/MHGAT.pdf}
%     \caption{Our framework with Multi-layer Multi-head Graph Convolution with Attention (MHGAT)}
%     \label{fig:mhgat}
% \end{figure}

In contrast to the graph convolution operation (Equation \ref{eq:norm_adj}), here we transform the initial input features through the multi-head attention network which generates the automated collaborative embedding as follows:

\begin{equation}
    \mathcal{F}^{l+1} = \mathcal{F}^{l} + {\mathbin\Vert}_{h=1}^{nh} \sigma( \sum_{j \in \mathcal{N}_i} \alpha^k_{ij} \mathcal{W}^k \mathcal{F}^l_j )
\end{equation}
where $\alpha^k_{ij}$ is normalized attention coefficients computed as follows:

\begin{equation}
    \alpha^k_{ij} = \frac{\exp( LeakyReLU ( \Vec{a}^T [\mathcal{W}\mathcal{F}_i \mathbin\Vert \mathcal{W} \mathcal{F}_j]))} {\sum_{k \in \mathcal{N}_i} \exp ( LeakyReLU (\Vec{a}^T [\mathcal{W}\mathcal{F}_i \mathbin\Vert \mathcal{W} \mathcal{F}_k]))}
\end{equation}

where $\mathbin\Vert$ represents concatenation, and $\Vec{a}^T$ denotes transpose of $\Vec{a} \in \mathbb{R}^{2f}$ which is implemented as a single-layer feed-forward neural network \cite{gat, gatv2}. 

Finally, after passing the $\mathcal{F}^{l+1}$ through a fully connected layer, we obtain the user and services embedding, consecutively the predicted QoS matrix as follows:  
\begin{equation}
    \mathcal{F}_u ~ \lvert \rvert_{r} ~ \mathcal{F}_s = \mathcal{F} ~~;~~ \quad 
    \mathcal{\hat{Q}} = \mathcal{F}_u \cdot \mathcal{F}_s
\end{equation}

The training-testing set-up of the MhGAT is kept the same as MhGCMF whose details are provided in Table \ref{tab:mhgat_parameters}. 

\subsection{Configuration of Various Networks}
In this subsection, we provide the configuration details of various parameters utilized in our framework. 

\subsubsection{Parameters Details for Autoencoders}\label{sec:autoencoder}
The configuration details of the autoencoders (AEs) used for the dimensionality reduction to generate initial feature embedding for users and services are presented in Table \ref{tab:autoencoder_config}. 
We use four AEs in total to generate the latent representation of the collaborative features using correlation and a one-hot representation of contextual information of users and services.
Two AEs (denoted as User-AE), used to generate user features, share the same configuration. 
% Similarly, the two AEs (denoted as Service-AE) used to extract the service features have identical configurations.
Similarly, to extract service features, two AEs (represented by Service-AE) with identical configurations are used.

\begin{table}[!h]\tiny
    \centering
    \caption{Configurations of Autoencoders}
    \begin{tabular}{l|c|c|c|c}
        \hline
        \multirow{2}{*}{\textbf{Parameters}} & \multicolumn{2}{c|}{\textbf{Configuration of User-AE}} & \multicolumn{2}{c}{\textbf{Configuration of Service-AE}}\\
        \cline{2-5}
        & $Encoder$ & $Decoder$ & $Encoder$ & $Decoder$\\ \hline \hline 
        {No. of layers} & 3 & 3 & 3 & 3  \\ \hline
        {No. of nodes} & 120; 80; 50 & 80; 120; 507 & 1000; 250; 50 & 250; 1000; 8598 \\ \hline
        {Activation functions~} & $\mathscr{T}$; $\mathscr{T}$; $\ell$ & $\mathscr{T}$; $\mathscr{T}$; $\ell$ &  $\mathscr{T}$; $\mathscr{T}$; $\ell$ & $\mathscr{T}$; $\mathscr{T}$; $\ell$ \\ \hline
        {Epoch} & \multicolumn{2}{c|}{500} &  \multicolumn{2}{c}{500} \\ \hline
        {Loss function} & \multicolumn{2}{c|}{MSE} & \multicolumn{2}{c}{MSE} \\ \hline
        {Optimizer} & \multicolumn{2}{c|}{RMSProp} & \multicolumn{2}{c}{RMSProp} \\ \hline
        {Dropout} & 0.6; 0.4 & 0.6; 0.4 & 0.6; 0.4 & 0.6; 0.4\\ \hline
        Patience parameter & \multicolumn{2}{c|}{\multirow{2}{*}{3}} &  \multicolumn{2}{c}{\multirow{2}{*}{3}}  \\ %\hline
        (Early stopping) & \multicolumn{2}{c|}{} &  \multicolumn{2}{c}{} \\ \hline
        Epochs	& \multicolumn{2}{c|}{500} &  \multicolumn{2}{c}{500} \\ \hline
        \multicolumn{5}{r}{\emph{Activation functions}: $\mathscr{T}$: tanh ; $\ell$: linear}   %\\
    \end{tabular}
    \label{tab:autoencoder_config}
\end{table}

\subsubsection{Parameters Details for MhGCMF}\label{subsec:gcn_details}
The configuration details for the MhGCMF are presented in Table \ref{tab:mhgcmf_parameters}.

\begin{table}[!h]\tiny
    \centering
    \caption{MhGCMF Parameters}
    \begin{tabular}{l|l|l}
    \hline
        \textbf{Parameters} &  \multicolumn{2}{c}{\textbf{Values}} \\ \hline \hline
        \multirow{2}{*}{Dense layers}
        & No. of layers & 1 \\ \cline{2-3}
        & Units &  128 $\times$ $N_h$  \\ \hline
        \multirow{4}{*}{GCMFU}
        & No. of units & 2 \\ \cline{2-3}
        & No. of heads ($N_h$) & 1-8 \\\cline{2-3}
        & Dimension of weight matrix ($W_1$) & 155 $\times$ 128 \\ \cline{2-3}
        & Dimension of weight matrix ($W_2$) & 128 $\times$ 64 \\ \hline
        \multirow{6}{*}{Conv}
        & Type & Conv 1D \\ \cline{2-3}
        & No. of units & 3\\ \cline{2-3}
        & No. of filters & 1 \\ \cline{2-3}
        & Filter size & 1$\times$1 \\ \cline{2-3}
        & Padding & same\\ \cline{2-3}
        & Stride & 1 \\ \hline
        Dimension of automated feature vector & $E_{fo}$ & 64\\ \hline
        \multirow{2}{*}{Optimizer} 
        & \multicolumn{2}{c}{Adam} \\ \cline{2-3}
        & Learning rate & 0.001 \\ \hline
        \multirow{2}{*}{Loss Function} 
        & \multicolumn{2}{c}{Cauchy} \\ \cline{2-3}
        & $\gamma$ for RT & 0.25\\ \cline{2-3}
        & $\gamma$ for TP & 10 \\ \hline
        Activation Function & 	 \multicolumn{2}{c}{ReLU} \\ \hline
        Patience parameter (Early stopping) &  \multicolumn{2}{c}{300} \\ \hline
        Epochs	&  \multicolumn{2}{c}{20000} \\ \hline
    \end{tabular}
    \label{tab:mhgcmf_parameters}
\end{table}

\subsubsection{Parameters Details for MhGAT}\label{subsec:gat_details}
The configuration details for the MhGAT are presented in Table \ref{tab:mhgat_parameters}.
\begin{table}[!h]\tiny
    \centering
    \caption{MhGAT Parameters}
    \begin{tabular}{l|l|l}
    \hline
        \textbf{Parameters} &  \multicolumn{2}{c}{\textbf{Values}} \\ \hline \hline
        \multirow{4}{*}{GAT} 
        & No. of units & 2 \\ \cline{2-3}
        & No. of heads ($N_h$) & 1-8 \\\cline{2-3}
        & Dimension of weight matrix & 155 $\times$ 128 \\ \cline{2-3}
        & Dimension of Weight attention matrix & 256 $\times$ 1 \\ \hline
        \multirow{6}{*}{Conv}
        & Type & Conv 1D \\ \cline{2-3}
        & No. of units & 3\\ \cline{2-3}
        & No. of filters & 1 \\ \cline{2-3}
        & Filter size & 1$\times$1 \\ \cline{2-3}
        & Padding & same\\ \cline{2-3}
        & Stride & 1 \\ \hline
        Dense layers 1 & Units &  128 $\times$ $N_h$  \\ \hline
        Dense layers 2 & Units &  64  \\ \hline
        Dimension of automated feature vector & $E_{fo}$ & 64\\ \hline
        \multirow{2}{*}{Optimizer} 
        & \multicolumn{2}{c}{Adam} \\ \cline{2-3}
        & Learning rate & 0.001 \\ \hline
        \multirow{2}{*}{Loss Function} 
        & \multicolumn{2}{c}{Cauchy} \\ \cline{2-3}
        & $\gamma$ for RT & 0.25\\ \cline{2-3}
        & $\gamma$ for TP & 10 \\ \hline
        Activation Function & 	 \multicolumn{2}{c}{ReLU} \\ \hline
        Patience parameter (Early stopping) &  \multicolumn{2}{c}{300} \\ \hline
        Epochs	&  \multicolumn{2}{c}{20000} \\ \hline
    \end{tabular}
    \label{tab:mhgat_parameters}
\end{table}

\subsubsection{Parameters Details for MLPs}\label{sec:mlp_details}
The configuration details for the MLPs used in the grey sheep and cold start modules are presented in Table \ref{tab:mlp_parameters}.
\begin{table}[!h]
    \centering
    \caption{MLP Parameters}
    \begin{tabular}{l|l|l}
    \hline
        \textbf{Parameters} &  \multicolumn{2}{c}{\textbf{Values}} \\ \hline \hline
        \multirow{2}{*}{Dense layers}
        & No. of layers & 3 \\ \cline{2-3}
        & Units &  128; 50; 1  \\ \hline
        Optimizer & \multicolumn{2}{c}{Adam} \\\hline
        \multirow{2}{*}{Loss Function} 
        & \multicolumn{2}{c}{Cauchy} \\ \cline{2-3}
        & $\gamma$ for RT & 0.25\\ \cline{2-3}
        & $\gamma$ for TP & 10 \\ \hline
        Activation Function & 	 \multicolumn{2}{c}{Sigmoid} \\ \hline
        Patience parameter (Early stopping) &  \multicolumn{2}{c}{3} \\ \hline
        Epochs &  \multicolumn{2}{c}{500} \\ \hline
        Batch size & \multicolumn{2}{c}{32} \\ \hline
    \end{tabular}
    \label{tab:mlp_parameters}
\end{table}
