# Supplementary material for: ARRQP: Anomaly Resilient Real-time QoS Prediction Framework with Graph Convolution
Source: arXiv:2310.02269 source file (2023-09-22)
Supplement: Supplementary file 2 [file 7AppendixNew.tex]

\section{Appendix-A}\label{sec:appendixA}
In this section, we provide the configuration details of various parameters utilized in our framework. 

\subsubsection{Parameters Details for MhGCMF}\label{subsec:gcn_details}
Table \ref{tab:mhgcmf_parameters} shows the configuration of the MhGCMF.

\begin{table}[!h]\tiny
    \centering
    \caption{MhGCMF Parameters}
    \begin{tabular}{l|l|l}
    \hline
        \textbf{Parameters} &  \multicolumn{2}{c}{\textbf{Values}} \\ \hline \hline
        \multirow{2}{*}{Dense layers}
        & No. of layers & 1 \\ \cline{2-3}
        & Units &  128 $\times$ $N_h$  \\ \hline
        \multirow{4}{*}{GCMFU}
        & No. of units & 2 \\ \cline{2-3}
        & No. of heads ($N_h$) & 1-8 \\\cline{2-3}
        & Dimension of weight matrix ($W_1$) & 155 $\times$ 128 \\ \cline{2-3}
        & Dimension of weight matrix ($W_2$) & 128 $\times$ 64 \\ \hline
        \multirow{6}{*}{Conv}
        & Type & Conv 1D \\ \cline{2-3}
        & No. of units & 3\\ \cline{2-3}
        & No. of filters & 1 \\ \cline{2-3}
        & Filter size & 1$\times$1 \\ \cline{2-3}
        & Padding & same\\ \cline{2-3}
        & Stride & 1 \\ \hline
        Dimension of automated feature vector & $E_{fo}$ & 64\\ \hline
        \multirow{2}{*}{Optimizer} 
        & \multicolumn{2}{c}{Adam} \\ \cline{2-3}
        & Learning rate & 0.001 \\ \hline
        \multirow{2}{*}{Loss Function} 
        & \multicolumn{2}{c}{Cauchy} \\ \cline{2-3}
        & $\gamma$ for RT & 0.25\\ \cline{2-3}
        & $\gamma$ for TP & 10 \\ \hline
        Activation Function & 	 \multicolumn{2}{c}{ReLU} \\ \hline
        Patience parameter (Early stopping) &  \multicolumn{2}{c}{300} \\ \hline
        Epochs	&  \multicolumn{2}{c}{20000} \\ \hline
    \end{tabular}
    \label{tab:mhgcmf_parameters}
\end{table}

\subsubsection{Parameters Details for MLPs}\label{sec:mlp_details}
The configuration details for the MLPs used in the grey sheep and cold start modules are presented in Table \ref{tab:mlp_parameters}.
\begin{table}[!h]
    \centering
    \caption{MLP Parameters}
    \begin{tabular}{l|l|l}
    \hline
        \textbf{Parameters} &  \multicolumn{2}{c}{\textbf{Values}} \\ \hline \hline
        \multirow{2}{*}{Dense layers}
        & No. of layers & 3 \\ \cline{2-3}
        & Units &  128; 50; 1  \\ \hline
        Optimizer & \multicolumn{2}{c}{Adam} \\\hline
        \multirow{2}{*}{Loss Function} 
        & \multicolumn{2}{c}{Cauchy} \\ \cline{2-3}
        & $\gamma$ for RT & 0.25\\ \cline{2-3}
        & $\gamma$ for TP & 10 \\ \hline
        Activation Function & 	 \multicolumn{2}{c}{Sigmoid} \\ \hline
        Patience parameter (Early stopping) &  \multicolumn{2}{c}{3} \\ \hline
        Epochs &  \multicolumn{2}{c}{500} \\ \hline
        Batch size & \multicolumn{2}{c}{32} \\ \hline
    \end{tabular}
    \label{tab:mlp_parameters}
\end{table}
